# Supplementary material for: Edge-aware Bidirectional Diffusion for Dense Depth Estimation from Light Fields
Source: arXiv:2107.02967 source file (2021-07-07)
Supplement: Supplementary file 1 [file results.tex]

\newcolumntype{x}[1]{%
>{\centering\hspace{0pt}}p{#1}}%

We present additional results on the real-world light fields from the Stanford dataset (17$\times$17). These light fields were captured using a camera-rig and have a larger baseline than synthetic or Lytro light fields. The light fields have been scaled down to half their original size. In the case of Jiang et al.~\cite{jiang2018} we could only use the central set of 7$\times$7 views as using all the 289 images caused their code to crash due to memory issues. Please see the accompanying video for a demonstration of the baseline of each light field, and our results.
\setlength{\tabcolsep}{1.5pt}

\begin{table}[t]
\begin{center}
\caption{The average reprojection error across the red, green, and blue channels for the four corner views of real world light fields set from Stanford. The error for each view is computed as the mean of the absolute difference between the real and reprojected view times $10^{-2}$. Overall, our method is comparable to state-of-the-art, and is significantly faster than the best non-learning-based method.}
\label{table:headings}
\vspace{-0.25cm}
\resizebox{0.8\linewidth}{!}{
\begin{tabular}{l|x{3em}x{3em}|x{3em}cc}
\hline
\multirow{2}{4em}{Light Field} & \multicolumn{2}{c}{Learning-based} & \multicolumn{3}{c}{Non-learning based} \\
\cline{2-6}
& \cite{shi2019} & \cite{jiang2018} & \cite{zhang2016} & \cite{jeon2015} & Ours\\
\hline
\textit{Bunny}  & \textbf{1.2} & 1.6 & 1.3 & 2.1 & \textbf{1.2} \\
\textit{Bulldozer} & \textbf{2.0} & 3.4 & \textbf{2.1} & 8.9 & 2.6 \\
\textit{Chess}  & \textbf{1.7} & \textbf{1.7} & \textbf{1.7} & 6.6 & \textbf{1.7}\\
\textit{Eucalyptus}   & \textbf{1.2} & 1.6 & 1.3 & 3.5 & \textbf{1.2}\\
\textit{Jelly-Beans} & \textbf{1.5} & 1.7 & \textbf{1.4} & 3.3 & 1.8 \\
\textit{Jewels} & \textbf{2.3} & 2.5 & 2.7 & 6.6 & \textbf{2.3} \\
\textit{Lego} & \textbf{2.5} & 4.4 & \textbf{3.1} & 7.6 & \textbf{3.1} \\
\textit{Tarot} & \textbf{9.9} & 17.2 & \textbf{15.2} & 20.1 & 17.8 \\
\textit{Truck} & \textbf{1.4} & 4.9 & 1.7 & 4.1 & \textbf{1.5} \\
\hline
\textit{\textbf{Average}} & \textbf{2.6} & 4.3 & \textbf{3.4} & 7.0 & 3.7 \\
\hline
\end{tabular}
}
\end{center}
\end{table}
\setlength{\tabcolsep}{1.4pt}

\setlength{\tabcolsep}{1.0pt}

\begin{table}[t]
\begin{center}
\caption{An evaluation of the running time of our algorithm on the 17$\times$17 real-world light fields of the Stanford dataset.
}
\vspace{-0.25cm}
\label{table:headings}
\resizebox{0.8\linewidth}{!}{
\begin{tabular}{l|x{3em}x{3em}|x{3em}x{3em}c}
\hline
\multirow{2}{4em}{Light Field} & \multicolumn{5}{c}{Run time (s)} \\
\cline{2-6}
& \cite{shi2019} & \cite{jiang2018} & \cite{jeon2015} & \cite{zhang2016} & Ours\\
\hline
\textit{Bulldozer} & 66.6 & 169 & 1792 & 719 & \textbf{34.6} \\
\textit{Bunny} & 116 & 225 & 1926 & 1257 & \textbf{42.3} \\
\textit{Chess} & 64.0 & 246 & 2377 & 1255 & \textbf{44.3} \\
\textit{Eucalyptus} & 63.0 & 194 & 1969 & 744 & \textbf{35.2} \\
\textit{Jelly beans} & 32.6 & 111 & 1189 & 473 & \textbf{19.7} \\
\textit{Jewels} & 63.5 & 178 & 1930  & 743 & \textbf{37.7} \\
\textit{Lego} & 41 & 226 & 1937 & 956 & \textbf{41.8} \\
\textit{Tarot} & 41 & 211 & 2256 & 1018 & \textbf{38.9} \\
\textit{Truck} & 66 & 170 & 1745 & 689 & \textbf{33.8} \\
\hline
\textit{\textbf{Average}} & 61.5 & 192 & 1902 & 873 & \textbf{36.5} \\
\hline
\end{tabular}
}
\end{center}
\end{table}
\setlength{\tabcolsep}{1.4pt}

\begin{figure*}[t]
\centering
\includegraphics[width=\textwidth]{./Figures/results/supplemental/results-tarot.png}
\caption{\emph{Tarot}, a real-world light field scene with a highly specular object. \textbf{Top row, left to right:} The central view of the input light field, Jeon et al.~\cite{jeon2015}, Zhang et al.~\cite{zhang2016}. \textbf{Bottom row, left to right:} Jiang et al.~\cite{jiang2018} (learning-based), Shi et al.~\cite{shi2019} (learning-based), and ours. Notice how the learning-based method of Shi et al. hallucinates depth in the images on the cards in the background. Unlike the non-learning based methods of Jeon et al. and Zhang et al., our method is able to deal with the highly specular surface as the gradient-based EPI line-filtering stage (main paper, Section 3.1) allows us to discard lines on the specular orb, yielding a depth that is almost piece-wise constant.} 
\label{fig:results-tarot}
\end{figure*}

\begin{figure*}[t]
\centering
\includegraphics[width=\textwidth]{./Figures/results/supplemental/err-tarot.png}
\caption{A visualization of the average reprojection error to the four corner views using the generated depth map. \textbf{Top row, left to right:} The central view of the input light field, Jeon et al.~\cite{jeon2015}, Zhang et al.~\cite{zhang2016}. \textbf{Bottom row, left to right:} Jiang et al.~\cite{jiang2018} (learning-based), Shi et al.~\cite{shi2019} (learning-based), and ours} 
\label{fig:results-tarot}
\end{figure*}

\begin{figure*}[t]
  \centering
  \includegraphics[width=\textwidth]{./Figures/results/supplemental/results-bunny.png}
  \caption{\emph{Bunny} real-world light field scene. \textbf{Top row, left to right:} The central view of the input light field, Jeon et al.~\cite{jeon2015}, Zhang et al.~\cite{zhang2016}. \textbf{Bottom row, left to right:} Jiang et al.~\cite{jiang2018} (learning-based), Shi et al.~\cite{shi2019} (learning-based), and ours. Notice the artifacts caused by disocclusions around the Bunny's face in the learning-based methods of Jiang et al., and Shi et al.}
  \label{fig:results-bunny}
\end{figure*}

\begin{figure*}[t]
  \centering
  \includegraphics[width=\textwidth]{./Figures/results/supplemental/err-bunny.png}
  \caption{A visualization of the average reprojection error to the four corner views using the generated depth map. \textbf{Top row, left to right:} The central view of the input light field, Jeon et al.~\cite{jeon2015}, Zhang et al.~\cite{zhang2016}. \textbf{Bottom row, left to right:} Jiang et al.~\cite{jiang2018} (learning-based), Shi et al.~\cite{shi2019} (learning-based), and ours}
  \label{fig:results-bunny}
\end{figure*}

\begin{figure*}[t]
  \centering
  \includegraphics[width=\textwidth]{./Figures/results/supplemental/results-bulldozer.png}
  \caption{\emph{Bulldozer} real-world light field scene. \textbf{Top row, left to right:} The central view of the input light field, Jeon et al.~\cite{jeon2015}, Zhang et al.~\cite{zhang2016}. \textbf{Bottom row, left to right:} Jiang et al.~\cite{jiang2018} (learning-based), Shi et al.~\cite{shi2019} (learning-based), and ours}
  \label{fig:results-bulldozer}
\end{figure*}

\begin{figure*}[t]
  \centering
  \includegraphics[width=\textwidth]{./Figures/results/supplemental/err-bulldozer.png}
  \caption{A visualization of the average reprojection error to the four corner views using the generated depth map. \textbf{Top row, left to right:} The central view of the input light field, Jeon et al.~\cite{jeon2015}, Zhang et al.~\cite{zhang2016}. \textbf{Bottom row, left to right:} Jiang et al.~\cite{jiang2018} (learning-based), Shi et al.~\cite{shi2019} (learning-based), and ours}
  \label{fig:results-bulldozer}
\end{figure*}

\begin{figure*}[t]
  \centering
  \includegraphics[width=\textwidth]{./Figures/results/supplemental/results-chess.png}
  \caption{\emph{Chess} real-world light field scene. \textbf{Top row, left to right:} The central view of the input light field, Jeon et al.~\cite{jeon2015}, Zhang et al.~\cite{zhang2016}. \textbf{Bottom row, left to right:} Jiang et al.~\cite{jiang2018} (learning-based), Shi et al.~\cite{shi2019} (learning-based), and ours}
  \label{fig:results-chess}
\end{figure*}

\begin{figure*}[t]
  \centering
  \includegraphics[width=\textwidth]{./Figures/results/supplemental/err-chess.png}
  \caption{A visualization of the average reprojection error to the four corner views using the generated depth map. \textbf{Top row, left to right:} The central view of the input light field, Jeon et al.~\cite{jeon2015}, Zhang et al.~\cite{zhang2016}. \textbf{Bottom row, left to right:} Jiang et al.~\cite{jiang2018} (learning-based), Shi et al.~\cite{shi2019} (learning-based), and ours}
  \label{fig:results-chess}
\end{figure*}

\begin{figure*}[t]
  \centering
  \includegraphics[width=\textwidth]{./Figures/results/supplemental/results-eucalyptus.png}
  \caption{\emph{Eucalyptus} real-world light field scene. \textbf{Top row, left to right:} The central view of the input light field, Jeon et al.~\cite{jeon2015}, Zhang et al.~\cite{zhang2016}. \textbf{Bottom row, left to right:} Jiang et al.~\cite{jiang2018} (learning-based), Shi et al.~\cite{shi2019} (learning-based), and ours}
  \label{fig:results-eucalyptus}
\end{figure*}

\begin{figure*}[t]
  \centering
  \includegraphics[width=\textwidth]{./Figures/results/supplemental/err-eucalyptus.png}
  \caption{A visualization of the average reprojection error to the four corner views using the generated depth map. \textbf{Top row, left to right:} The central view of the input light field, Jeon et al.~\cite{jeon2015}, Zhang et al.~\cite{zhang2016}. \textbf{Bottom row, left to right:} Jiang et al.~\cite{jiang2018} (learning-based), Shi et al.~\cite{shi2019} (learning-based), and ours}
  \label{fig:results-eucalyptus}
\end{figure*}

\begin{figure*}[t]
  \centering
  \includegraphics[width=\textwidth]{./Figures/results/supplemental/results-jelly-beans.png}
  \caption{\emph{Jelly-Beans} real-world light field scene. \textbf{Top row, left to right:} The central view of the input light field, Jeon et al.~\cite{jeon2015}, Zhang et al.~\cite{zhang2016}. \textbf{Bottom row, left to right:} Jiang et al.~\cite{jiang2018} (learning-based), Shi et al.~\cite{shi2019} (learning-based), and ours}
  \label{fig:results-jelly-beans}
\end{figure*}

\begin{figure*}[t]
  \centering
  \includegraphics[width=\textwidth]{./Figures/results/supplemental/err-jelly-beans.png}
  \caption{A visualization of the average reprojection error to the four corner views using the generated depth map. \textbf{Top row, left to right:} The central view of the input light field, Jeon et al.~\cite{jeon2015}, Zhang et al.~\cite{zhang2016}. \textbf{Bottom row, left to right:} Jiang et al.~\cite{jiang2018} (learning-based), Shi et al.~\cite{shi2019} (learning-based), and ours}
  \label{fig:results-jelly-beans}
\end{figure*}

\begin{figure*}[t]
  \centering
  \includegraphics[width=\textwidth]{./Figures/results/supplemental/results-jewels.png}
  \caption{\emph{Jewels} real-world light field scene. \textbf{Top row, left to right:} The central view of the input light field, Jeon et al.~\cite{jeon2015}, Zhang et al.~\cite{zhang2016}. \textbf{Bottom row, left to right:} Jiang et al.~\cite{jiang2018} (learning-based), Shi et al.~\cite{shi2019} (learning-based), and ours}
  \label{fig:results-jewels}
\end{figure*}

\begin{figure*}[t]
  \centering
  \includegraphics[width=\textwidth]{./Figures/results/supplemental/err-jewels.png}
  \caption{A visualization of the average reprojection error to the four corner views using the generated depth map. \textbf{Top row, left to right:} The central view of the input light field, Jeon et al.~\cite{jeon2015}, Zhang et al.~\cite{zhang2016}. \textbf{Bottom row, left to right:} Jiang et al.~\cite{jiang2018} (learning-based), Shi et al.~\cite{shi2019} (learning-based), and ours}
  \label{fig:results-jewels}
\end{figure*}

\begin{figure*}[t]
\centering
\includegraphics[width=\textwidth]{./Figures/results/supplemental/results-lego.png}
\caption{\emph{Lego} real-world light field scene. \textbf{Top row, left to right:} The central view of the input light field, Jeon et al.~\cite{jeon2015}, Zhang et al.~\cite{zhang2016}. \textbf{Bottom row, left to right:} Jiang et al.~\cite{jiang2018} (learning-based), Shi et al.~\cite{shi2019} (learning-based), and ours}
\label{fig:results-lego}
\end{figure*}

\begin{figure*}[t]
\centering
\includegraphics[width=\textwidth]{./Figures/results/supplemental/err-lego.png}
\caption{A visualization of the average reprojection error to the four corner views using the generated depth map. \textbf{Top row, left to right:} The central view of the input light field, Jeon et al.~\cite{jeon2015}, Zhang et al.~\cite{zhang2016}. \textbf{Bottom row, left to right:} Jiang et al.~\cite{jiang2018} (learning-based), Shi et al.~\cite{shi2019} (learning-based), and ours}
\label{fig:results-lego}
\end{figure*}

\begin{figure*}[t]
  \centering
  \includegraphics[width=\textwidth]{./Figures/results/supplemental/results-truck.png}
  \caption{\emph{Truck} real-world light field scene. \textbf{Top row, left to right:} The central view of the input light field, Jeon et al.~\cite{jeon2015}, Zhang et al.~\cite{zhang2016}. \textbf{Bottom row, left to right:} Jiang et al.~\cite{jiang2018} (learning-based), Shi et al.~\cite{shi2019} (learning-based), and ours}
  \label{fig:results-truck}
\end{figure*}

\begin{figure*}[t]
  \centering
  \includegraphics[width=\textwidth]{./Figures/results/supplemental/err-truck.png}
  \caption{A visualization of the average reprojection error to the four corner views using the generated depth map. \textbf{Top row, left to right:} The central view of the input light field, Jeon et al.~\cite{jeon2015}, Zhang et al.~\cite{zhang2016}. \textbf{Bottom row, left to right:} Jiang et al.~\cite{jiang2018} (learning-based), Shi et al.~\cite{shi2019} (learning-based), and ours}
  \label{fig:results-truck}
\end{figure*}
