# Supplementary material for: Edge-aware Bidirectional Diffusion for Dense Depth Estimation from Light Fields
Source: arXiv:2107.02967 source file (2021-07-07)
Supplement: Supplementary file 7 [file fig-results-jewels.tex]

\begin{figure*}[t]
  \centering
  \includegraphics[width=\textwidth]{./Figures/results/supplemental/results-jewels.png}
  \caption{\emph{Jewels} real-world light field scene. \textbf{Top row, left to right:} The central view of the input light field, Jeon et al.~\cite{jeon2015}, Zhang et al.~\cite{zhang2016}. \textbf{Bottom row, left to right:} Jiang et al.~\cite{jiang2018} (learning-based), Shi et al.~\cite{shi2019} (learning-based), and ours}
  \label{fig:results-jewels}
\end{figure*}

\begin{figure*}[t]
  \centering
  \includegraphics[width=\textwidth]{./Figures/results/supplemental/err-jewels.png}
  \caption{A visualization of the average reprojection error to the four corner views using the generated depth map. \textbf{Top row, left to right:} The central view of the input light field, Jeon et al.~\cite{jeon2015}, Zhang et al.~\cite{zhang2016}. \textbf{Bottom row, left to right:} Jiang et al.~\cite{jiang2018} (learning-based), Shi et al.~\cite{shi2019} (learning-based), and ours}
  \label{fig:results-jewels}
\end{figure*}
