# Supplementary material for: Edge-aware Bidirectional Diffusion for Dense Depth Estimation from Light Fields
Source: arXiv:2107.02967 source file (2021-07-07)
Supplement: Supplementary file 9 [file fig-results-tarot.tex]

\begin{figure*}[t]
\centering
\includegraphics[width=\textwidth]{./Figures/results/supplemental/results-tarot.png}
\caption{\emph{Tarot}, a real-world light field scene with a highly specular object. \textbf{Top row, left to right:} The central view of the input light field, Jeon et al.~\cite{jeon2015}, Zhang et al.~\cite{zhang2016}. \textbf{Bottom row, left to right:} Jiang et al.~\cite{jiang2018} (learning-based), Shi et al.~\cite{shi2019} (learning-based), and ours. Notice how the learning-based method of Shi et al. hallucinates depth in the images on the cards in the background. Unlike the non-learning based methods of Jeon et al. and Zhang et al., our method is able to deal with the highly specular surface as the gradient-based EPI line-filtering stage (main paper, Section 3.1) allows us to discard lines on the specular orb, yielding a depth that is almost piece-wise constant.} 
\label{fig:results-tarot}
\end{figure*}

\begin{figure*}[t]
\centering
\includegraphics[width=\textwidth]{./Figures/results/supplemental/err-tarot.png}
\caption{A visualization of the average reprojection error to the four corner views using the generated depth map. \textbf{Top row, left to right:} The central view of the input light field, Jeon et al.~\cite{jeon2015}, Zhang et al.~\cite{zhang2016}. \textbf{Bottom row, left to right:} Jiang et al.~\cite{jiang2018} (learning-based), Shi et al.~\cite{shi2019} (learning-based), and ours} 
\label{fig:results-tarot}
\end{figure*}
