# Supplementary material for: Edge-aware Bidirectional Diffusion for Dense Depth Estimation from Light Fields
Source: arXiv:2107.02967 source file (2021-07-07)
Supplement: Supplementary file 11 [file normals.tex]

\subsection{Normal Maps}
\label{sec:appendix_normals}

Figure~\ref{fig:normal-maps-a} and Figure~\ref{fig:normal-maps-b} show the normal maps estimated from the depth output of each method on the HCI dataset. In general, while our output tends to be less noisy than the learning-based method of Li et al~\cite{li2020}, quantization artifacts resulting from weighted median filtering can be seen in our results and those of Zhang et al.~\cite{zhang2016}. Increasing the quantization levels may improve these, at the cost of a longer running time. 

\begin{figure*}
\centering
\includegraphics[width=\textwidth]{Figures/supplemental/normals-a.pdf}
\caption{Normal maps for the HCI dataset.  } 
\label{fig:normal-maps-a}
\end{figure*}

\begin{figure*}
\centering
\includegraphics[width=\textwidth]{Figures/supplemental/normals-b.pdf}
\caption{Normal maps for the HCI dataset.  } 
\label{fig:normal-maps-b}
\end{figure*}
